# Supplementary material for: Reflection Measurement of the Scattering Mean Free Path at the Onset of Multiple Scattering
Source: arXiv:2401.02246 source file (2024-09-10)

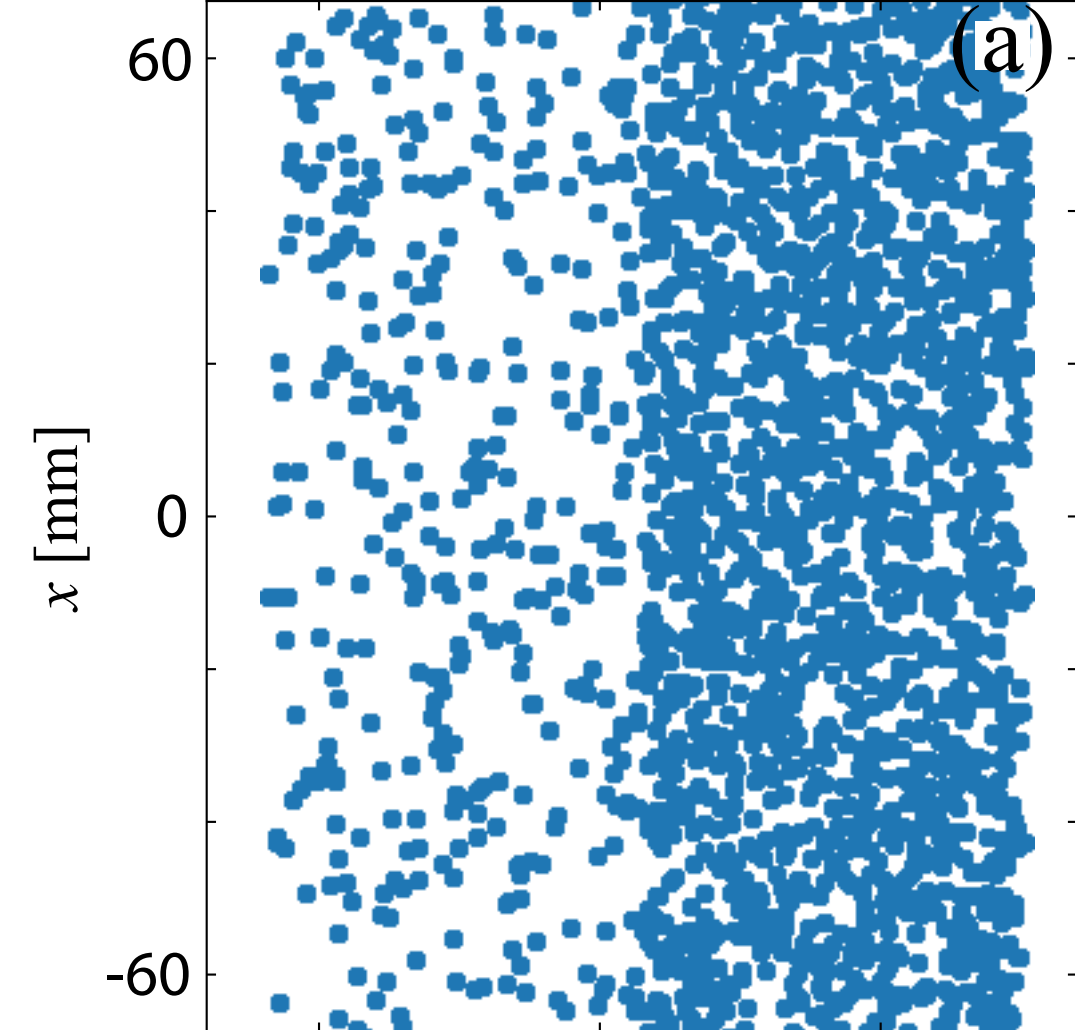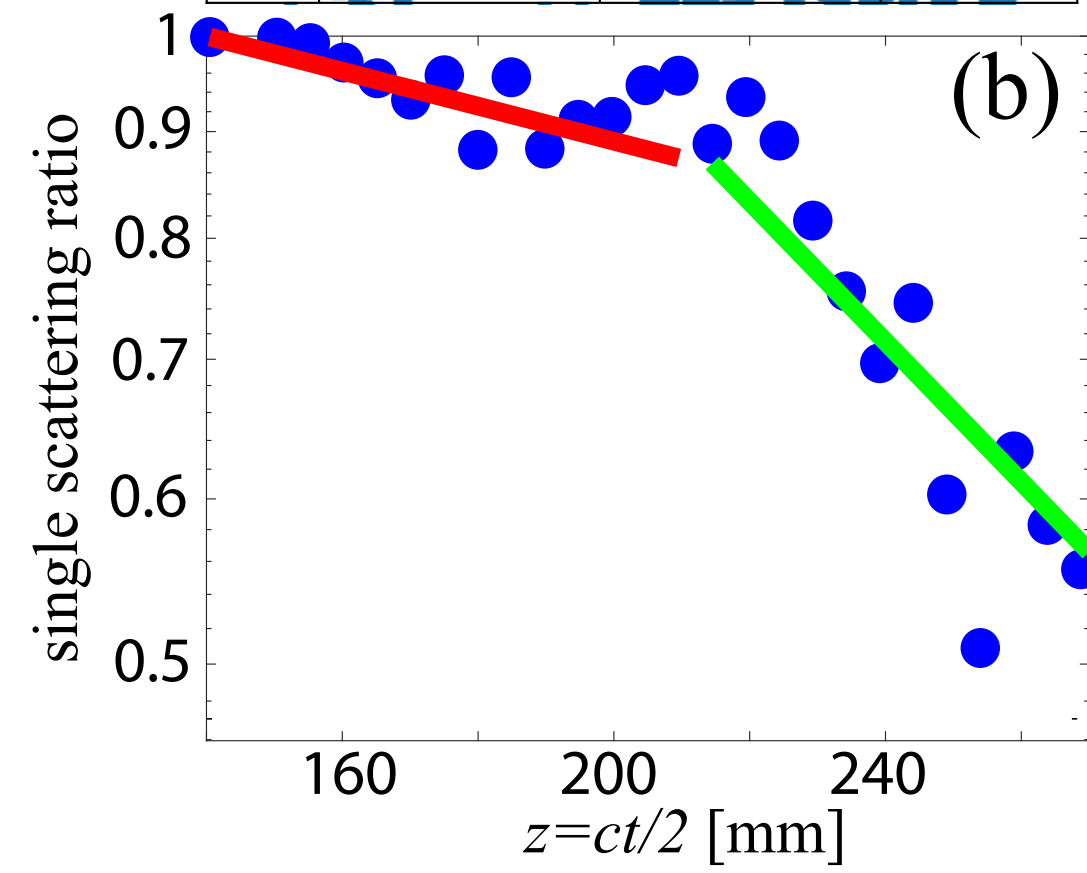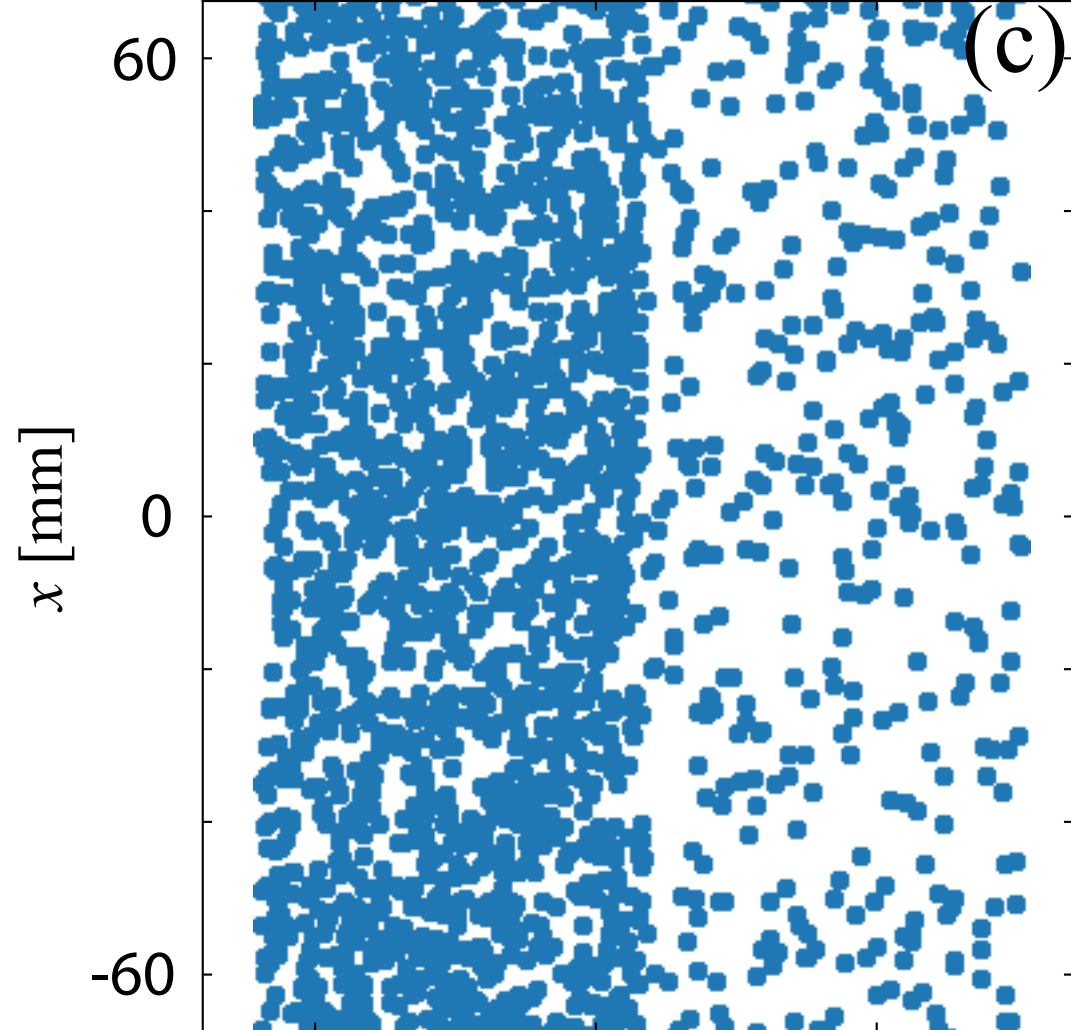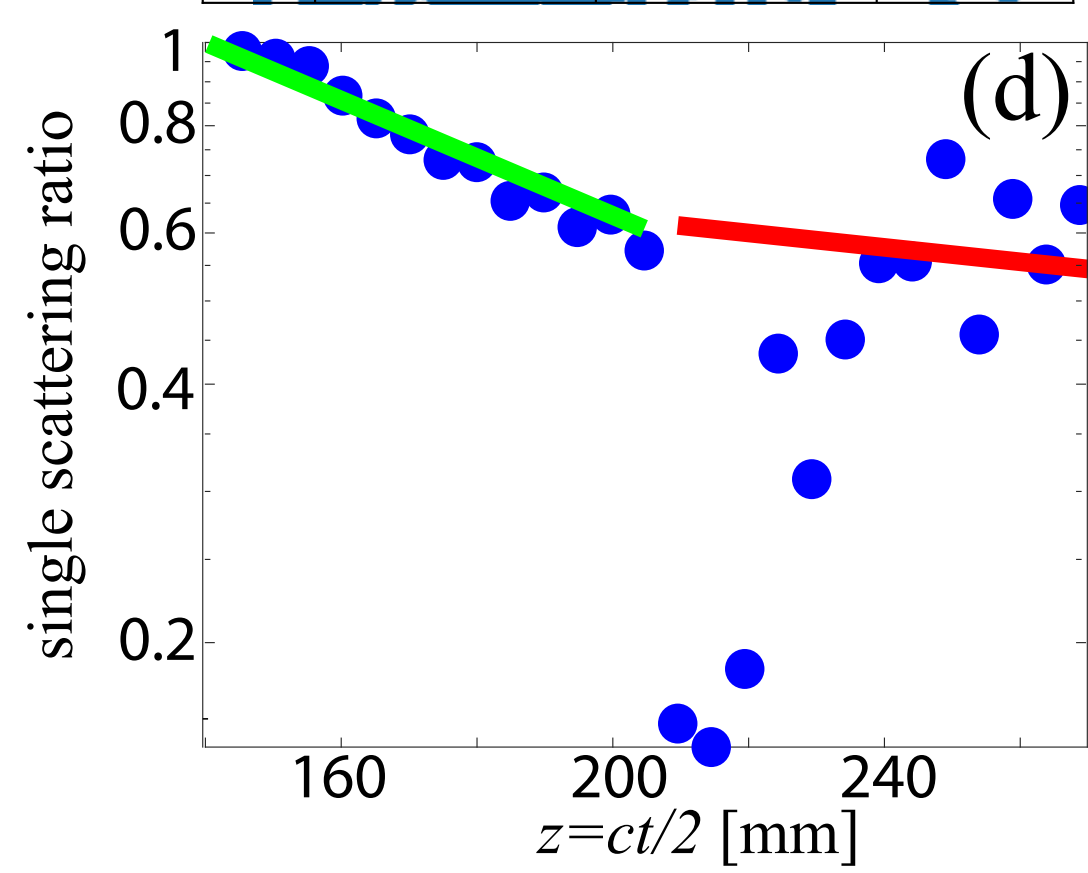

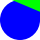

(d)

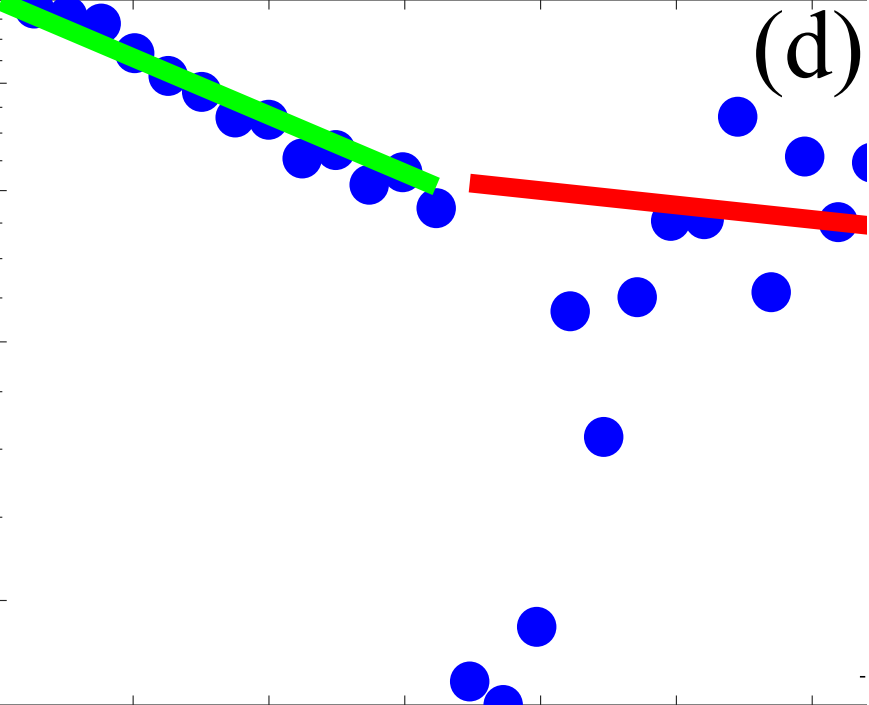

(d)

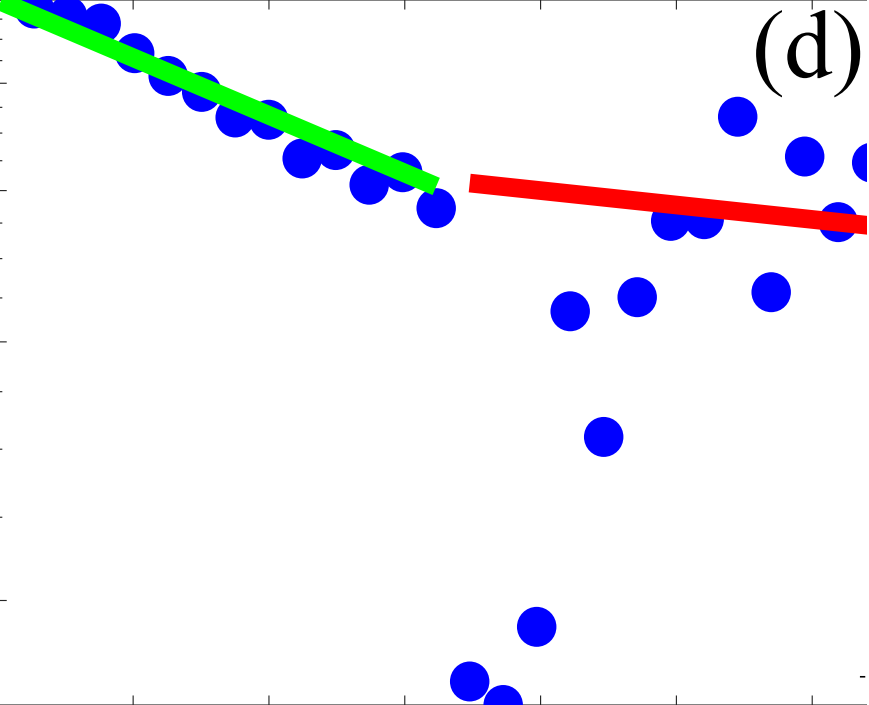

Supplement: Supplementary file 1 [file figure_sm_2dens-2.pdf]
